# Supplementary material for: Hamiltonian path and Hamiltonian cycle are solvable in polynomial time in graphs of bounded independence number
Source: arXiv:2309.09228 source file (2025-04-01)
Supplement: Supplementary file 1 [file appendix.tex]

\section{Hamiltonian linkage}\label{sec:linkage-in-appendix}

\subsection{Definitions}

The formal definition of the computational problems we are interested in is this:

\computationproblem{{\sc Hamiltonian-$\ell$-Linkage}}{A graph $G$ and distinct vertices $s_1,\ldots,s_{\ell},t_1,\ldots,t_{\ell}\in V(G)$.}{Does there exist a Hamiltonian linkage for $s_1,\ldots,s_{\ell},t_1,\ldots,t_{\ell}$ in $G$?}

%\medskip\noindent
%{\sc Hamiltonian-$\ell$-Linkage}\\
%Input: A graph $G$ and distinct vertices $s_1,\ldots,s_{\ell},t_1,\ldots,t_{\ell}\in V(G)$.\\
%Question: Does there exist a Hamiltonian linkage for $s_1,\ldots,s_{\ell},t_1,\ldots,t_{\ell}$ in $G$?

\computationproblem{{\sc Hamiltonian-$\ell$-Linkedness}}{A graph $G$.}{Is $G$ Hamiltonian-$\ell$-linked? }

\computationproblem{{\sc $\ell$-Path-Cover}}{A graph $G$.}{Do there exist distinct vertices   $s_1,\ldots,s_{\ell},t_1,\ldots,t_{\ell}\in V(G)$ and a Hamiltonian linkage for them in $G$?}

\subsection{Proofs of NP-hardness results for Hamiltonian linkage in general graphs}

\begin{proof} {\bf of Theorem~\ref{thm:HL-NPc}}.
Let $G$ be a connected graph, subject to the question if it contains a Hamiltonian path. Construct $G'$ by adding $2\ell$ new extra vertices $s_1, \ldots, s_{\ell}, t_1,\ldots, t_{\ell}$ and edges $s_1s_i, s_it_i$ and $t_it_1$ for all $ i=2,\ldots,\ell$ and $s_1v,t_1v$ for all  $v\in E(G)$. In any linkage of $s_1,\ldots,t_{\ell}$ (not necessarily a Hamiltonian one), the vertices $s_i,t_i$, $i=2,3,\ldots,\ell$ are linked via the edge $s_it_i$, since any other path in $G'$ connecting these vertices would pass through $s_1$ and $t_1$ and these two vertices could not be linked. Thus $s_1$ and $t_1$ must be linked via a path in $G$, which must visit all vertices of $G$ if the linkage is Hamiltonian. It follows that $s_1,\ldots,t_{\ell}$ are Hamiltonian linked in $G'$ if and only if $G$ contains a Hamiltonian path.   
\end{proof}

\begin{proof} {\bf of Theorem~\ref{thm:NPhard-PathCover}}.
Let $G$ be a connected graph, subject to the question if it contains a Hamiltonian path. Construct $G'$ by adding $\ell+3$ new extra vertices $a,b,c,d_1,\ldots,d_{\ell}$ and edges $au, u\in V(G)$, $ab,bc$ and $cd_i, i=1,2,\ldots,\ell$. In any path cover, at most two of the vertices $d_i, i=1,2,\ldots,\ell$ belong to the same path, since such a path passes through vertex $c$. If this is the case, then a path cover by $\ell$ can be achieved only by making all vertices of $V(G)\cup\{a,b\}$ be covered by a single path, which would have to start in $b$, and this is possible only if (and if) $G$ itself contains a Hamiltonian path. If each vertex $d_i, i=1,2,\ldots,\ell$ belongs to a different path, we have already $\ell$ of them, and so one of them must pass through $c, b$ and $a$ and continue as a Hamiltonian path in $G$. Thus $G'$ can be covered by at most $\ell$ paths if and only if $G$ contains a Hamiltonian path, and the path cover number of $G'$ is exactly $\ell$ in such a case.
\end{proof}

\begin{proof} {\bf of Theorem~\ref{thm:HLinkedness-NPc}}.
Let us first briefly argue that for a fixed $\ell$, the {\sc Hamiltonian-$\ell$-Linkedness} problem is in NP, though it asks about the existence of Hamiltonian linkage {\em for any} collection of $\ell$ pairs of vertices of the input graph. For {\sc Hamiltonian-$\ell$-Linkage}, the guess-and-verify certificate to prove NP-membership is simply a collection of $\ell$ paths connecting the need-to-be-linked vertices, including checking that every vertex of the input graph belongs to exactly one of these paths. For   {\sc Hamiltonian-$\ell$-Linkedness}, a guess-and-verify certificate is a list of $O(n^{2\ell})$ such collections of paths, where $n$ is the order of the input graph. For a fixed $\ell$, this is a polynomial-time verifiable certificate.

Now we prove the NP-hardness by a reduction from {\sc $\ell$-Path-Cover} which is NP-complete according to Theorem~\ref{thm:NPhard-PathCover}. Given an input graph $G$ with $n$ vertices subject to the question if $G$ can be covered by $\ell$ disjoint paths, we may assume that $n>3\ell$, since we can solve the problem by brute force (which would still take only $O(1)$ time) otherwise. We construct a graph $G'$ by adding $2\ell$ new extra vertices $x_1,\ldots,x_{2\ell}$ to $G$, and making each of them adjacent to all vertices of $G$. (Formally, $V(G')=V(G)\cup  X$, where $X=\{x_1,\ldots,x_{2\ell}\}$, and $E(G')=E(G)\cup\{xu: x\in X, u\in V(G)\}$.) We claim that $G'$ is Hamiltonian-$\ell$-linked if and only if $G$ can be covered by $\ell$ disjoint paths.

For the ``only if'' direction, suppose that $G'$ is Hamiltonian-$\ell$-linked. Then the vertices $s_i=x_i, t_i=x_{\ell+i}, i=1,2,\ldots,\ell$ are Hamiltonian linked in $G'$, and in such a linkage, each path $P_i=s_i\ldots t_i$ induces a path $A_i=P_i\cap V(G)$ in $G$ and these paths form a path cover of $G$.

The proof of the ``if'' part is slightly more involved. Suppose $G$ can be covered by $\ell$ disjoint paths $A_1,\ldots,A_{\ell}$. We will show that any collection of vertices $s_1,\ldots,t_{\ell}$ in $G'$ are Hamiltonian linked in $G'$. Let $s_1,\ldots,t_{\ell}\in V(G')$ be such a collection, for the sake of brevity, we will call these vertices {\em marked}. Let $k$ of the pairs $s_i,t_i$ have both vertices in $X$ and let $h$ of them have only one vertex in $X$. The remaining $\ell-k-h$ pairs have both vertices in $V(G)$. That means that $X$ has $2\ell-2k-h$ vertices which are not marked, and we will call these vertices {\em free}.         

For each path $A_i$, choose its orientation from left to right and partition its vertices into {\em segments} in the following way: For every marked vertex $u\in V(A_i)$, the segment $S(u)$ contains $u$ and the maximal subpath of $A_i$ which contains vertices to the left of $u$ and for which $u$ is the only marked vertex of this segment. If the right end-vertex of the path $A_i$ is not marked, we create one more segment containing the vertices lying on $A_i$ to the right from its right-most marked vertex, and we call this segment {\em free}.

Having done this with all paths $A_i,i=1,2,\ldots,\ell$, we get the vertices of $G$ partitioned into $2\ell-2k-h$ marked segments and at most $\ell$ free ones. Now we modify the segments so that we have exactly $\ell$ of the free ones. Since $n>3\ell$, we have at least $\ell$ vertices in $G$ which are not marked. Some of them will be taken away from their segments and pronounced single-vertex free segments so that the all the segments are paths in $G$, they form a partition of $V(G)$, there are exactly $\ell$ free segments and every marked segment is either a single marked vertex or a path containing exactly one marked vertex, which is then an endpoint of this segment. To achieve this, we simply remove the necessary number of unmarked vertices from their former segments from left to right.

Finally we show how to build a Hamiltonian linkage for the marked vertices. For a pair of marked vertices $s_i,t_i\in X$, choose a free segment $S$ in $G$ and take the path $P_i=s_i,S,t_i$ (and delete $S$ from the pool of free segments). For a pair of marked vertices $s_i,t_i$ such that exactly one of them, say $s_i$, is in $X$, tak the path $P_i=s_i,S(t_i)$. For a pair of marked vertices $s_i,t_i\in V(G)$, choose a free vertex $x\in X$ and take the path $P_i=S(s_i)^{-1},x,S(t_i)$. Having done this for all $i=1,\ldots,\ell$, we have created disjoint paths $P_i,i=1,2,\ldots,\ell$ in $G'$, and these paths contain all vertices of $G'$ except for $2\ell-2k-h-(\ell-k-h)=\ell-k$ free vertices of $X$ (say, $y_1,\ldots,y_{\ell-k}$) and $\ell-k$ free segments in $G$ (which were not used so far, say $S_1,\ldots,S_{\ell-k}$). The path $P_1$ contains two consecutive vertices $u\in X, v\not\in X$ (or  $u\not\in X, v\in X$, which is analogous) and we modify $P_1$ by inserting the sequence $S_1,y_1,S_2,y_2,\ldots,S_{\ell-k},y_{\ell-k}$ between $u$ and $v$. Now the paths $P_1,\ldots,P_{\ell}$ form a path cover of $G'$. This concludes the proof.    
\end{proof}

\subsection{Hamiltonian linkage for graphs of bounded independence number}\label{subsec:main-appendix}

We start with a formal definition of a scenario.

\begin{definition}
Let $G$ be a graph, let $A\subset V(G)$ be a vertex cut and let $Q_1,\ldots,Q_s$ be the connected components of $G-A$. Let $s_1,\ldots,s_{\ell}, t_1,\ldots,t_{\ell}$ be distinct vertices of $G$. A {\em scenario} for $s_i,t_i$ is a sequence of vertices of $G$ starting with $s_i$ and ending with $t_i$ such that no two consecutive elements belong to different components $Q_i,Q_j$ and no three consecutive elements belong to the same component $Q_i$ (in other words, between any two closest occurrences of vertices from $A$, there are at most 2 vertices from the components $Q_i$, and if they are 2, then they are from the same component). A {\em collection of scenarios} for $s_1,\ldots,s_{\ell}, t_1,\ldots,t_{\ell}$ is a set $\cal S$ of $\ell$ scenarios $S_1,\ldots,S_{\ell}$ such that for each $i$, $S_i$ is a scenario for $s_i,t_i$. A scenario collection ${\cal S}=\{S_1,\ldots,S_{\ell}\}$ is {\em plausible} if every vertex of $A$ belongs to exactly one scenario $S_i$ and appears only once in it, every vertex of $G-A$ belongs to at most one scenario $S_i$ and appears only once in it, and in every scenario $S_i$, any two consecutive elements that do not both belong to the same component $Q_j$ are adjacent in $G$.  
\end{definition}

Now we describe the main algorithm and its {\bf Reduce} subroutine in a pseudocode:

\begin{algorithm}
\caption{$HamLinkage(G,k,\ell, s_1,\ldots,s_{\ell},t_1,\ldots,t_{\ell})$.}\label{alg:algorithm}
\begin{algorithmic}[1]
\Require A graph $G$, a non-negative integer $\ell$, distinct vertices $s_1,\ldots,s_{\ell},t_1,\ldots,t_{\ell}\in V(G)$.
\Ensure \texttt{true} if $G$ contains a Hamiltonian linkage for $s_1,\ldots,s_{\ell},t_1,\ldots,t_{\ell}$, \texttt{false} otherwise.
\If{$\ell=0$ and $V(G)\neq\emptyset$}
    \State \Return \texttt{false}
\EndIf
\If{$\ell=0$ and $V(G) = \emptyset$}
    \State \Return \texttt{true}
\EndIf
\State \textbf{compute} the vertex connectivity $c_v(G)$ of $G$ and a minimum vertex cut $A\subseteq V(G)$
\If{$c_v(G)\ge g(k,\ell)$} 
		\State \Return \texttt{true}
	\Else
		\State \textbf{denote}  by $Q_i, i=1,2,\ldots,s$ the connected components of $G-A$;
		\State $HamLinked \gets$ \texttt{false}
		\ForAll {plausible scenario collections $\cal S$ $=\{S_1,S_2,\ldots,S_{\ell}\}$}
			\State $GoodScenario \gets$ \texttt{true}
			\For{$i = 1, \dots, s$}
				\State $Reduce(Q_i,{\cal S},Q',\ell', s'_1,\ldots,t'_{\ell'})$
				\If{$HamLinkage(G[Q'],k-1,\ell',s'_1,\ldots,t'_{\ell'})=$ \texttt{false}}
					\State $GoodScenario \gets$ \texttt{false}
				\EndIf
			\EndFor
			\If{$GoodScenario$}
					\State $HamLinked \gets$ \texttt{true}
			\EndIf		
		\EndFor 
		\If {$HamLinked$}
			\State \Return \texttt{true}
		\Else 
			\State \Return \texttt{false}
		\EndIf
\EndIf 
\end{algorithmic}
\end{algorithm}

\begin{algorithm}
\caption{$Reduce(Q,{\cal S},Q',\ell',s'_1,\ldots,t'_{\ell'})$.}\label{alg:subroutine}
\begin{algorithmic}[1]
\Require A connected component $Q$ of $G-A$, a plausible scenario collection ${\cal S}=\{S_1,\ldots,S_{\ell}\}$ for $s_1,\ldots,t_{\ell}$.
\Ensure  A subset $Q'\subseteq Q$, an integer $\ell' \geq 0$, distinct vertices $s'_1,\ldots,s'_{\ell'},t'_1,\ldots,t'_{\ell'}\in Q'$.
\State $Q' \gets Q$; $\ell' \gets 0$
\For{ $i=1, \ldots, l$}
	\ForAll {$u\in S_i\cap Q$ such that no neighbor of $u$ on $S_i$ belongs to $Q$}
		\State $Q'\gets Q'\setminus\{u\}$
	\EndFor	
	\ForAll { $u,v\in Q$ that are distinct and appear consecutively on $S_i$}
		\State $\ell'\gets \ell'+1$; $s'_{\ell'}\gets u$; $t'_{\ell'}\gets v$
	\EndFor	
\EndFor
\State \Return $(Q',\ell',s'_1,\ldots,t'_{\ell'})$

\end{algorithmic}
\end{algorithm}

\begin{lemma}
Algorithm~\ref{alg:algorithm} correctly answers if a $kK_1$-free graph contains a Hamiltonian linkage for the input vertices $s_1,\ldots,t_{\ell}$. 
\end{lemma}

\begin{proof}
The correctness has been argued upon in the outline of the algorithm. We will justify the $Reduce$ subroutine. The correspondence between a path $P$ and its scenario $S$ is such that if two consecutive vertices of $S$ belong to the same component $Q_i$, they correspond to a path connecting these vertices in $G[Q_i]$ as a subpath of $P$. Therefore these two vertices are added as a pair to the need-to-be-linked vertices for the recursive call. If there is only one vertex of $Q_i$ between two vertices from $A$ on $S$, say $a_1,q,a_2$ are consecutive vertices with $a_1,a_2\in A, q\in Q_i$, then $a_1,q,a_2$ is a subpath of $P$ and vertex $q$ cannot be used by any other path of the linkage. Therefore we delete this vertex from $Q_i$ for the recursive call. It is then clear that a collection of scenarios can be realized by a linkage of the need-to-be-linked vertices if and only if it is plausible and the recursive calls on the reduced components all return value {\texttt{true}}. And that the vertices can be linked if and only if there exists at least one plausible scenario collection that can be realized by a linkage. 
\end{proof}

\begin{proof} {\bf of Corollary~\ref{cor:vsechnopolynomialni}}.
Set $\ell=1$ in Theorem~\ref{thm:Ham-linkage-poly} and check all pairs of vertices of the input graph if this pair is Hamiltonian linked. This can be done in time $O(n^{2+f(k,1)})$. The graph contains a Hamiltonian path if the answer is ``yes" for at least one pair of vertices, it contains a Hamiltonian cycle if the answer is ``yes" for at least one pair of adjacent vertices, and it is Hamiltonian connected if the answer is ``yes" for all the pairs. 
\end{proof}

\begin{proof} {\bf of Corollary~\ref{cor:pathcover}}.
It is obvious that $\mathrm{pc}(G)\le \alpha(G)$. (Consider an optimal collection of $\mathrm{pc}(G)$ paths that cover all vertices and take one end-vertex from each of the paths. These vertices must form an independent set, since if any two of them were adjacent, these two paths could be replaced by their concatenation to form a cover by $\mathrm{pc}(G)-1$ paths. Thus $\alpha(G)\ge \mathrm{pc}(G)$.) If we assume that $G$ is $kK_1$-free, it suffices to call {\sc $\ell$-Path-Cover} on $G$ for $\ell=1,2,\ldots,k-1$ and return the smallest value of $\ell$ for which we get an affirmative answer. Hence the path cover number can be determined in time $O(k\cdot n^{f(k,k-1)})=  O(n^{f(k,k-1)}).$ 
\end{proof}

\section{Omitted proofs for graphs with small independence number}

\subsection{$3K_1$-free graphs}

\begin{proof} \textbf{of Theorem~\ref{thm:3K1_uv}.} Clearly, if at least one of the conditions is violated, then $G$ does not have a Hamiltonian path $P_{u,v}$.

Assume that all of the conditions are satisfied and $G$ is connected but not 2-connected. Then there exists an articulation point $x$. Since $G$ is $3K_1$-free, $G-\{x\}$ has exactly 2 connected components. Let us denote them by $Q_1, Q_2$. Since $G$ is $3K_1$-free, both of the components are cliques, $x$ is adjacent to all vertices of at least one clique, say $Q_2$, and $x$ is adjacent to at least one vertex, say $x'$, in the other clique $Q_1$. 

The vertex $x$ is different from $u,v$ by (a) and $u,v$ are in different components of $G-\{x\}$ by (b), say $u$ is in $Q_1$ and $v$ is in $Q_2$. If $u=x'$ and $|Q_1|>1$, there is another vertex $x''\in Q_1$ adjacent to $x$ because $u$ is not an articulation point. We obtain a Hamiltonian path $P_{u,v}$ by concatenating a path in $G[Q_1]$ starting in vertex $u$, passing through all vertices of $Q_1$ and ending in $x'$ (or in $x''$, if $u=x'$ and $|Q_1|>1$) with a path $P_{x,v}$ in $G[Q_2\cup \{x\}]$ passing through all vertices of $Q_2$ and ending in vertex $v$.

Now assume that $G$ is $2$-connected but not $3$-connected. We will use a similar approach as in \cite{chvatal1972note}. Take a longest path $P$ from $u$ to $v$ and suppose for a contradiction that this is not a Hamiltonian path. Then there exists a vertex $x \in V(G) \setminus V(P)$ and since $G$ is 2-connected, $P$ contains at least 3 vertices. By Proposition~\ref{prop:menger}, there exist vertices $y_1,y_2$ (ordered in the direction from $u$ to $v$) on $P$ together with internally disjoint paths $P_1,P_2$ from $x$ to $y_1,y_2$. If $y_1,y_2$ are consecutive on $P$, then we obtain a longer path by replacing the edge $y_1y_2$ by the concatenation of the paths $P^{-1}_1$ and $P_2$, contradicting the maximality of $P$. Thus we assume that no two disjoint paths from $x$ to $P$ end in consecutive vertices of $P$.

If $y_1=u$ and $y_2=v$ and there is no path from $x$ to $V(P)$ ending in a vertex different from $u$ and $v$, then $\{u,v\}$ is a vertex cut in $G$, violating condition (c). Hence we may choose $y_1,y_2$ so that at least one of them is not an and-vertex of $P$. Assume without loss of generality that $y_2 \neq v$ (the other case is symmetric). Denote by $y_1'$ the successor of $y_1$ and by $y_2'$ the successor of $y_2$ on the path $P$ (in the direction from $u$ to $v$). Then $xy_1', xy_2'$ are not edges in $G$, otherwise we would have a longer path. Since $G$ is $3K_1$-free, $y_1'y_2'$ is an edge. But then the path obtained by concatenating the subpath of $P$ from $u$ to $y_1$, $P_1^{-1}$, $P_2$, the subpath of $P^{-1}$ from $y_2$ to $y_1'$, the edge $y_1'y_2'$ and the subpath of $P$ from $y_2'$ to $v$, is a path from $u$ to $v$ and longer than $P$, a contradiction. 

If $G$ is at least 3-connected, then it is Hamiltonian connected by Proposition~\ref{prop:chvatal}. 
\end{proof}

\begin{proof} \textbf{of Theorem~\ref{thm:3K1u}.}
If $u$ is an articulation point then such Hamiltonian path does not exist. 

Suppose that $u$ is not an articulation point and that $G$ is connected but not 2-connected. There is an articulation point $x$ in $G$ and $x \neq u$. The graph $G-\{x\}$ has exactly two components and they are cliques. We construct a Hamiltonian path starting at vertex $u$, going through all vertices of the clique containing $u$ to a neighbour of $x$ (note that either $u$ is the only vertex in its component, or $x$ is adjacent to another vertex in this component, since $u$ would be an articulation point otherwise), moving through $x$ to the other component and then traversing the vertices of the other clique in an arbitrary order.

If $G$ is at least 2-connected, then it has a Hamiltonian cycle by Proposition~\ref{prop:chvatal}, thus it has a Hamiltonian path starting at any vertex.
\end{proof}

\begin{proof} \textbf{of Theorem~\ref{thm:3K1pathcover}.}
If $G$ has a Hamiltonian path starting at vertex $u$, then it has also a $\mathrm{PC}(u,v)$. Assume that there is no Hamiltonian path starting at vertex $u$ and thus, $u$ is an articulation point by Theorem~\ref{thm:3K1u}. Since the components of $G-\{u\}$ are cliques, we can obtain one path starting at $v$ going through the component in which $v$ is contained and the other path starting at $u$, moving to an adjacent vertex in the other component and then traversing all of its vertices in an arbitrary order.
\end{proof}

\subsection{$4K_1$-free graphs}

\begin{proof} \textbf{of Theorem~\ref{thm:4k1}.}
If $G$ is at least 2-connected, then $G$ has a Hamiltonian path by Proposition~\ref{prop:chvatal}, and also both (a) and (b) are satisfied.

Suppose that $G$ is connected but not 2-connected. If there exists an articulation $x$ such that $G-\{x\}$ has at least 3 components (see Figure~\ref{fig:4k1}a), then $G$ cannot have a Hamiltonian path. Since $G$ is a $4K_1$-free graph, there cannot be more than 3 components and if there are exactly 3 components, then all of them must be cliques. Clearly, in this case, the path cover number of $G$ is equal to 2. 

From now on assume that for each articulation $x$, $G-\{x\}$ has at most 2 components. Let $x$ be an articulation and $Q_1$, $Q_2$ be two non-empty components of $G-\{x\}$. Then at least one of $Q_1$ and $Q_2$, say $Q_1$, must be a clique and the other one, hence $Q_2$, must induce a $3K_1$-free graph.

Observe, that $G$ has a Hamiltonian path if and only if $G[Q_2]$ has a Hamiltonian path starting at some vertex $u \in Q_2$ adjacent to $x$,  and that happens if and only if $u$ is not an articulation point in $G[Q_2]$ (by Theorem~\ref{thm:3K1u}). 

Suppose that all neighbours of $x$ in $Q_2$ are articulation points of $G[Q_2]$. 
Let $y \in Q_2$ be such a vertex. Both components of $G[Q_2]-\{y\}$ are cliques, $y$ is adjacent to all vertices of at least one component and to at least one vertex in the other one, say $y'$. The vertices $y$ and $y'$ are the only possible articulation points in $G[Q_2]$, and thus $x$ is non-adjacent to all vertices of $Q_2$ except $y$ and possibly $y'$. If $x$ is not adjacent to $y'$, then $c(G-\{y\}) \geq 3$ and condition (a) is violated. If $x$ and $y'$ are adjacent, $y'$  is also an articulation point of $G[Q_2]$ and $y$ and $y'$ are the only neighbours of $x$ in $Q_2$. Then $x,y,y'$ form a triangle in $G$ such that $G-\{x,y,y'\}$ has at least 3 components and condition (b) is violated. In this case, all components of $G-\{x,y,y'\}$ are cliques and $G$ clearly has a path cover of size 2. See Figure~\ref{fig:4k1} as an illustration of these two cases.

Thus, if both conditions (a) and (b) are satisfied, then we  obtain a Hamiltonian path in $G$ by concatenating a Hamiltonian path in clique $G[Q_1]$, $x$ and a Hamiltonian path of $G[Q_2]$ starting in a neighbour $u \in {Q_2}$ of $x$. 
\end{proof}

\begin{proof} \textbf{of Theorem~\ref{thm:4k1_1con}.}
Clearly, if any of the conditions is not satisfied, then $G$ does not have a Hamiltonian path starting at vertex $u$. 

Suppose that all of the conditions (a)--(f) are satisfied.

\textit{Case 1. $G$ is connected, but not $2$-connected.}

Let $x$ be an articulation point of $G$. Then one of the components of $G-\{x\}$ is a clique, say $Q_1$, and the other one, say $Q_2$,  is a $3K_1$-free graph. 

\textit{Case 1a. $G[Q_2]$ is not connected.} This cannot happen, since otherwise $G-\{x\}$ has at least 3 components and that would violate condition (a).

\textit{Case 1b. $G[Q_2]$ is connected, but not 2-connected.} 
If $u \in Q_1$, then $G$ has a Hamiltonian path if and only if $x$ has a neighbour in $Q_2$ which is not an articulation point of $G[Q_2]$ (by Theorem~\ref{thm:3K1u}). Such a neighbour always exists, otherwise condition (a) would be violated. 

Suppose that $u \in Q_2$. If $u$ is an articulation point of $G[Q_2]$, then $c(G-\{u,x\}) \geq 3$ and condition (e) would be violated. Thus, $u$ is not an articulation point of $G[Q_2]$. %pridane
For every articulation point $y$ of $G[Q_2]$, $G[Q_2] - \{y\}$ has at most two components and they are cliques. Moreover, by condition (c), $x$ has a neighbour $x'$ in the component of $G[Q_2] - \{y\}$ which does not contain $u$ such that $x'$ is not an articulation point of $G[Q_2]$. %pridane
Thus, there exists a Hamiltonian path of $Q_2$ from $u$ to $x'$ by Theorem~\ref{thm:3K1_uv} and we can concatenate it with a Hamiltonian path of the clique $G[Q_1]$ to obtain a Hamiltonian path of $G$. 

\textit{Case 1c. $G[Q_2]$ is 2-connected, but not 3-connected.} 
If $u \in Q_1$, then a Hamiltonian path in $G$ can be easily obtained by concatenating a Hamiltonian path in $G[Q_1]$ starting at $u$, vertex $x$ and a Hamiltonian cycle of $G[Q_2]$ (it exists by Proposition~\ref{prop:chvatal}). 

If $u \in Q_2$, then $G$ has a Hamiltonian path if and only if $G[Q_2]$ has a Hamiltonian path starting in vertex $u$ and ending in a neighbour of $x$. By Theorem~\ref{thm:3K1_uv}, such a Hamiltonian path exists if there exists a neighbour $v$ of $x$ such that $\{u,v\}$ do not form a vertex cut of size two in $G[Q_2]$. Non-existence of such neighbour would violate condition (d). 

\textit{Case 1d. $G[Q_2]$ is at least 3-connected.} In this case, $G[Q_2]$ is Hamiltonian connected which implies the existence of a Hamiltonian path in $G$. 

\textit{Case 2. $G$ is $2$-connected, but not $3$-connected.} 

If there exists a vertex cut $\{x,y\}$ such that $c(G- \{x,y \}) \geq 3$. Since $G$ is $4K_1$-free, $c(G-\{x,y\})>3$ cannot happen. Hence $c(G-\{x,y\}) = 3$ and 
all components of $G-\{x,y\}$ are cliques. Condition (e) implies that $u\neq x,y$. But then it is easy to see that $G$ has 
a Hamiltonian path starting in vertex $u$.

Assume from now on that for any vertex cut $\{x,y\}$ we have $c(G- \{x,y \}) =2$, and consider such a cut $\{x,y\}$. Again, one of the components of $G- \{x,y \}$ is a clique, say $Q_1$, and the other one, say $Q_2$,  induces a $3K_1$-free subgraph of $G$. It follows that $G[Q_2]$ contains at most 2 articulation points, and if it contains two of them, then they are adjacent.  Denote by $X$ ($Y$) the neighbourhood of $x$ (of $y$, respectively) in $Q_2$. Observe that if there exists a Hamiltonian path in $G[Q_2]$ starting in a vertex from $X$ and ending in a vertex from $Y$, then $G$ has a Hamiltonian cycle, and thus it has a Hamiltonian path starting in any vertex. If $|X\cup Y|=1$, it must be $|Q_2|=1$ and $G$ contains a Hamiltonian cycle. Let further $|Q_2|>1$, and hence also $|X\cup Y|>1$. If there is no Hamiltonian path in $G[Q_2]$ starting in a vertex from $X$ and ending in a vertex from $Y$, then one of the conditions of Theorem~\ref{thm:3K1_uv} must be violated for any choice of different vertices, one from $X$ and the other one from $Y$. 

\textit{Case 2a. $X$ or $Y$ contains only articulation points of $G[Q_2]$.} Since $G$ is $2$-connected, only one of $X,Y$ can contain only articulation points, say $X$. 
Denote the components of $G[Q_2] \setminus X $ as $A$ and $B$. Since $G[Q_2]$ is $3K_1$-free, $X$ contain at most two vertices. Let $a \in X$ be a vertex adjacent to a vertex in $A$ and let $b \in X$ be a vertex adjacent to a vertex in $B$ (it is possible that $a=b$).
Observe that $x$ must be adjacent to all vertices in $Q_1$. Otherwise, $x$, its non-neighbour in $Q_1$, a vertex from $A$ and a vertex from $B$ would form a $4K_1$.

The vertex $y$ must have at least one neighbour in $A$ and  at least one neighbour in $B$ such that they are not articulation points in $G[Q_2]$. If $u \in Q_1$, we obtain a Hamiltonian path starting in vertex $u$, going through all vertices of $Q_1$, $x$, $a$, all vertices in $A$ ending in a vertex adjacent to $y$, $y$ and all vertices in $B$.  
If $u=x$, then we obtain a Hamiltonian path starting in $x$ going through all vertices of $Q_1$, $y$ and a Hamiltonian path of $Q_2$ starting in a vertex in $Y$ which is not an articulation point of $G[Q_2]$. If $u=y$, then condition (f) would be violated. If $u \in Q_2$ and $u$ is not an articulation point of $G[Q_2]$, then we obtain a Hamiltonian path starting in vertex $u$ by concatenating a Hamiltonian path of $G[Q_2]$ starting in $u$ and ending in a neighbour of $y$ (such a path always exists by condition (f) and  Theorem~\ref{thm:3K1_uv}) with a Hamiltonian path of $G[Q_1\cup\{x,y\}]$ starting in $y$ and ending in $x$. Finally, suppose that $u \in Q_2$ and $u$ is an articulation point in $G[Q_2]$. If $u$ is the only neighbour of $x$ in $Q_2$, then $\{ y,u \}$ form a vertex cut such that $c(G- \{y,u \}) =3$. If $u$ is not the only neighbour of $x$ in $Q_2$ (say $u \neq a$), then we obtain a Hamiltonian path starting in vertex $u$, going through all vertices of $B$, $y$, all vertices of $Q_1$, $x$, $a$ and all vertices of $A$.

\textit{Case 2b. There is an articulation point $z$ in $G[Q_2]$ such that both $X$ and $Y$ are  subsets of one component of $G[Q_2]-\{z\}$.} This cannot happen, since $z$ would be an articulation point of entire $G$. 

\textit{Case 2c. $X \cup Y$ is a vertex cut in $Q_2$.} This also cannot happen, since  $G- \{x,y\}$ would have 3 components otherwise.   
\end{proof}

\begin{proof} \textbf{of Theorem~\ref{thm:4k1pc}.}
It is clear that if any of the conditions is not satisfied, then $\mathrm{PC}(u,v)$ does not exist. 

First suppose that $G$ is connected and  all of the conditions (a)--(d) are satisfied. If there exists a Hamiltonian path starting in $u$ (without loss of generality, we can interchange $u$ and $v$), then there is also a path cover $\mathrm{PC}(u,v)$. 

If such a path does not exist, then at least one of the conditions in Theorem \ref{thm:4k1_1con} is violated.  

\textit{Case 1: $G$ does not have a Hamiltonian path.} That means, that condition (a) of Theorem \ref{thm:4k1_1con} is violated. If $G$ does not have any Hamiltonian path, then by Theorem \ref{thm:4k1}, there exists an articulation point $x$, such that $G-\{x\}$ has at least 3 components or a triangle on articulation points $x,y,z$ in $G$ such that $c(G-\{x,y,z\}) \geq 3$. In both cases, there are exactly 3 components since $G$ is $4K_1$-free and they are cliques. 

\textit{Case 1a: There exists an articulation point $x$, such that $c(G-\{x\})  \geq 3$. } By condition (a) of this theorem we have that $x \neq u,v$ and $u,v$ are in different components of $G-\{x\}$. Denote the component containing $u$ by $Q_u$, the component containing $v$ by $Q_v$, and the third component by $Q_w$. If $u$ is the only neighbour of $x$ in $Q_u$ and $v$ is the only neighbour of $x$ in $Q_v$, then $\{u,v\}$ is a vertex cut in $G$ with $c(G-\{u,v\})\geq 3$. That would violate the condition (c) of this theorem. Thus, $x$ has at least two neighbours in at least one of $Q_u$, $Q_v$, say in $Q_u$. We can obtain the first path of $\mathrm{PC}(u,v)$ starting at $u$, traversing all the vertices of $Q_u$ (ending in a neighbour of $x$), then continuing to $x$ and then to all vertices of $Q_w$. The second path starts at $v$ and traverses all vertices of $Q_v$. 

\textit{Case 1b: There exists a triangle on articulation points $x,y,z$ in $G$ such that $c(G-\{x,y,z\}) \geq 3$.} 
Denote the component adjacent to $x$ by $Q_x$, the component adjacent to $y$ by  $Q_y$, and the component adjacent to $z$ by $Q_z$.  
First observe that $x$ is adjacent to all vertices in $Q_x$, otherwise $x$, a vertex from $Q_x$ not adjacent to $x$, a vertex from $Q_y$, and a vertex from $Q_z$ would create a $4K_1$. Analogously, $y$ is adjacent to all vertices in $Q_y$ and $z$ is adjacent to all vertices in $Q_z$.  

If both $u,v$ belong to $\{x,y,z\}$, then they would form a vertex cut such that $c(G-\{u,v\}) \geq 3$ and the condition (c) of this theorem would be violated. 

If exactly one of $u,v$ belongs to $\{x,y,z\}$, say $u=z$,  then we can obtain one path starting at $u$ traversing all vertices of $Q_z$ and the second path starting at $v$ and traversing all vertices of cliques $Q_x, Q_y$. 

If none of $u,v$ belongs to $\{x,y,z\}$ and they are in different components $G-\{x,y,z\}$, then it is clear that $G$ has a $\mathrm{PC}(u,v)$.

\textit{Case 2. The graph $G$ does have a Hamiltonian path, but does not have a Hamiltonian path starting neither in vertex $u$ nor $v$}. Several cases can occur, depending on which of the conditions (b)--(f) of Theorem~\ref{thm:4k1_1con} are violated.

\textit{Case 2a. The vertex $u$ is an articulation point of $G$}. That means that the condition (b) of Theorem~\ref{thm:4k1_1con} is violated. One of the components of $G-\{u\}$ is a clique, say $Q_1$, and the other one, say $Q_2$, induces a $3K_1$-free graph. 

First suppose that $v \in Q_1$. If all neighbours of $u$ in $Q_2$ are articulation points of $G[Q_2]$, then two situations can occur. Either there exists an articulation point $x \in {Q_2}$ such that  $c(G-\{x\}) \geq 3$ (in case $u$ has exactly one neighbour in $Q_2$). This is not possible. Or $u$ has two neighbours in $Q_2$ and the condition (b) of this theorem is violated. 

If $u$ has a neighbour, say $w$, in $Q_2$ which is not an articulation point of $G[Q_2]$, there exists a Hamiltonian path in $G[Q_2]$ starting in $w$. This can be extended to a Hamiltonian path of $G[Q_2\cup\{u\}]$ starting in $u$, which together with any Hamiltonian path in $G[Q_1]$ starting in vertex $v$ forms a $\mathrm{PC}(u,v)$.

Now suppose that $v \in Q_2$. 
If $v$ is an articulation point in $G[Q_2]$, then $G-\{u,v\}$ has at least 3 components, which is not possible (condition (c) of the theorem would be violated). If $v$ is not an articulation point of $G[Q_2]$, then there exists a Hamiltonian path of $G[Q_2]$ starting in $v$, which together with any Hamiltonian path of $G[Q_1\cup\{u\}]$ starting  vertex $u$ forms a path cover $\mathrm{PC}(u,v)$.

\textit{Case 2b. The condition (c) of Theorem~\ref{thm:4k1_1con} is violated.} 
Suppose that conditions (a)--(b) of Theorem~\ref{thm:4k1_1con} holds, thus $u$ is not articulation point of $G$. Let $x\neq u$ be an articulation point of $G$, let $Q_1$ be the component of $G-\{x\}$ containing $u$, and $Q_2$ be the other component of $G-\{x\}$. Suppose that $G[Q_1]$ contains an articulation $y\neq u$. Denote the components of $G[Q_1]-\{y\}$ by $J_1, J_2$. Suppose that $u \in J_1$ and $x$ is adjacent only to vertices from the component of $G[J_1] \cup \{y\}$. 

Note that $G[Q_2], G[J_1], G[J_2]$ are cliques and $x$ is adjacent to all vertices in at least one of $G[Q_2], G[J_1]$ (otherwise we would have a $4K_1$). 
We will distinguish several cases depending on the position of $v$. 
\begin{itemize}
\item 
If $v \in Q_2$ and there exists $x' \neq v \in Q_2$ adjacent to $x$, then we can obtain one path of $\mathrm{PC}(u,v)$ starting in $v$, traversing all vertices of $G[Q_2]$ (ending in $x'$), and ending in $x$. The second path is a Hamiltonian path of $G[Q_1]$ starting at $u$ (its existence being guaranteed by Theorem~\ref{thm:3K1u}). 

\item
Suppose that $v \in Q_2$ and $v$ is the only neighbour of $x$ in $G[Q_2]$. If $|Q_2| = 1$, then we can proceed as in the previous case. If $|Q_2| > 1$, then $x$ must be adjacent to all vertices in $J_1$, otherwise we would obtain a $4K_1$. 
\begin{itemize}
\item If $|J_1| = 1$ (it contains only vertex $u$) and $xy$ is not an edge, then $\{u,v\}$ forms a vertex cut in $G$ such that $c(G-\{u,v\})\geq 3$, which would violate condition (c) of this theorem. 
\item If $|J_1| = 1$ and $xy$ is an edge, then we can obtain one path starting at $u$ and traversing all vertices of $G[Q_2]$ and the second path traversing $u$, $x$, $y$, and all vertices if $G[J_2]$. 
\item Suppose $|J_1| > 1$. Take a Hamiltonian path of $G[Q_1]$ starting at $u$ and denote the first edge by $uu'$. Observe, that $u' \in J_1$ and thus $xu'$ is an edge. Replace $uu'$ by edges $ ux, xu'$. Take this path as one path of $\mathrm{PC}(u,v)$ and as the second path, take a path starting in $v$ traversing all vertices of $Q_2$.
\end{itemize}

\item
If $v = x$, then we can obtain one path of $\mathrm{PC}(u,v)$ starting in $v$, traversing all vertices of $G[Q_2]$ and the second path is a Hamiltonian path of $G[Q_1]$ starting at $u$.

\item
If $v \in J_1$, then each Hamiltonian path of $G$ must traverse vertices in this order (or in the reverse order): vertices of $Q_2$, $x$, vertices of $J_1$, $y$, vertices of $J_2$. Recall that $G[J_1]$ induces a clique. Our goal is to show, that there exists a Hamiltonian path of $G$ which traverses vertices of $G$ in this order: vertices of $Q_2$, $x$, some vertices of $J_1$, $u$, $v$ (or $v$,$u$), the rest of vertices of $J_1$, $y$, vertices of $J_2$. Obviously, this would give us a $\mathrm{PC}(u,v)$. 
Several cases can occur.
\begin{itemize}
\item 
If $x,y$ has exactly one common neighbour and no other neighbours in $J_1$, then the condition (a) or (b) of this theorem would be violated.
\item 
Suppose that $x$ is adjacent only to $u$ (and possibly also $v$) in $J_1$ and $y$ is adjacent only to $v$ (and possibly also $u$) in $J_1$ (or vice versa). If $xy$ is not an edge, then the condition (c) would be violated and if $xy$ is an edge, then the condition (d) would be violated. 
\item 
Without loss of generality (the situation for $y$ is symmetric), suppose that $x$  has a neighbour $x'$ in $J_1$ other than $u,v$, and $y'$ is a neighbour of $y$ other than $x'$ (possibly $y'=u$ or $y'=v$). We can traverse vertices in the order: $x$, $x'$, vertices of $J_1 \setminus \{x',y',u,v\}$ in an arbitrary order, $u$, $v$ (or vice versa), and finally $y'$ to get the sought Hamiltonian path. Note that it is possible $y'$ to be $u$ or $v$.  
\end{itemize}

\item  
If $v = y$, then we can obtain one path of $\mathrm{PC}(u,v)$ starting at $v$, traversing all the vertices of $J_2$. The problem arises if $u$ is the only neighbour of $x$ in $J_1$ and $|J_1|>1$. However, this cannot happen since $\{u,v\}$ would form a vertex cut in $G$ such that $c(G-\{u,v\})\geq 3$ and condition (c) would be violated. Thus, we can obtain the second path starting at $u$, traversing all the vertices of $G[J_1]$ (ending in a neighbour of $x$), continuing to $x$ and all the vertices of $G[Q_2]$. (The path can be shortened in the case $|J_1|=1$.)

\item 
If $v \in J_2$, then we can proceed as in the case of $v \in Q_2$ since the situation is symmetric (just the role of $x, Q_2$ and $y, J_2$ is interchanged).
\end{itemize}

\textit{Case 2c. The condition (d) of Theorem~\ref{thm:4k1_1con} is violated.}
Suppose that the conditions (a)-(c) of Theorem~\ref{thm:4k1_1con} hold. Let $x\neq u$ be an articulation point of $G$, let $Q_1$ be the component of $G-\{x\}$ containing $u$, $G[Q_1]$ is 2-connected, and let $Q_2$ be the other component. Suppose that for every $x' \in {Q_1}$ adjacent to $x$, $\{u,x'\}$ forms a minimal vertex cut of size two in $G[Q_1]$.
In other words, $G[Q_1]-\{u\}$ is not 2-connected and $x$ is in $Q_1$ adjacent only to the articulation points of $G[Q_1]-\{u\}$ (and possibly to $u$).

Since $G[Q_1]-\{u\}$ is not 2-connected, there exists an articulation point $y$ of $G[Q_1]-\{u\}$. Denote the components of $G[Q_1]-\{u,y\}$ by $J_1$, $J_2$. Since $G[Q_1]-\{u\}$ is $3K_1$-free, both $J_1$, $J_2$ are cliques, $y$ is adjacent to all vertices in one component of $G[Q_1]-\{u,y\}$, say $J_1$, and let $y'$ be a neighbour of $y$ in $J_2$. If $y'$ is the only neighbour of $y$ in $J_2$, then $y'$ is also an articulation point of $G[Q_1]-\{u\}$ and there are no other articulation points. Thus, $x$ can be adjacent only to $y$ or $y'$ (or both). 

Observe, that since $G$ is a $4K_1$-free graph, $x$ is adjacent to all vertices of $Q_2$. Recall that $G[Q_1]$ is 2-connected $3K_1$-free graph and thus, it has a Hamiltonian cycle. Several cases can occur depending on position of $v$. 
\begin{itemize}
\item 
If $v \in Q_2 \cup x$, then since $G[Q_2 \cup \{x\}]$ is a clique and $G[Q_1]$ has a Hamiltonian cycle, we are done. 
\item 
If $v \in J_1$, $v \neq y,y'$ (analogously if  $v \in J_2$), then one path starts at $v$ and traverses all vertices of $G[J_1]$ (except for $y'$ if $y'$ is the only neighbour of $x$ in $Q_1$). The second path starts at $u$, traverses all the vertices of $G[J_2]$, $y$, $x$, if $xy \in E(G)$, or $y',x$ otherwise, and then all the vertices of $G[Q_2]$.
\item  
If $v = y$ and $x$ is adjacent to $y'$ (analogously if $v = y'$) and $x$ is adjacent to $y$, then we proceed as in the previous case. 
\item 
If $v = y$ (analogously if $v = y'$) and $v$ is the only neighbour of $x$ in $Q_1$, then $\{u,v\}$ violates the condition (c).
\end{itemize}

\textit{Case 2d. The condition (e) of Theorem~\ref{thm:4k1_1con} is violated.} Suppose that the conditions (a)-(d) of Theorem~\ref{thm:4k1_1con} hold. There exists a vertex $x$ such that $c(G-\{u,x\}) \geq 3$. If $v=x$, then  condition (c) of this theorem is violated. 

Suppose that $v \neq x$. First suppose that $\{u,x\}$ is a minimal vertex cut of $G$. There are exactly 3 components, denote them by $Q_1, Q_2, Q_3$, of $G-\{u,x\}$ and all of them are cliques. Thus, $G$ is 2-connected and both $x$, $u$ has at least one neighbour in each component. Without loss of generality, let $v \in Q_1$. We can obtain one path of $\mathrm{PC}(u,v)$ starting at vertex $u$ and traversing all the vertices of $Q_1$. The second path starts at $u$, then traverses all the vertices of $Q_2$, $x$, and all the vertices $Q_3$. 

If $\{u,x\}$ is not a minimal vertex cut of $G$, then $x$ is an articulation point of $G$ ($u$ is not an articulation point, since (b) of Theorem~\ref{thm:4k1_1con} holds) and $G- \{x\}$ has at most 2 components (since (a) of Theorem~\ref{thm:4k1_1con} holds). Denote the component of $G- \{x\}$ containing $u$ by $Q_1$ and the other component by $Q_2$. The vertex $u$ is an articulation point of $G[Q_1]$. Denote the components of $G[Q_1]- \{u\}$ by $J_1$ and $J_2$. The vertex $u$ is adjacent to all vertices in at least one component, without loss of generality in $J_1$, and has at least one neighbour $u'$ in $J_2$.  Since $u$ is not an articulation point of $G$, then $x$ has a neighbour in both $J_1$, $J_2$. Several cases can occur depending on position of $v$. 
\begin{itemize}
\item 
If $v \in Q_2$, then one path of $\mathrm{PC}(u,v)$ starts at $v$ and traverses all the vertices of $G[Q_2]$. The second path starts at $u$, traverses all the vertices of $G[J_1]$, $x$, and all the vertices of $G[J_2]$. 
\item 
If $v \in J_2$, then one path of $\mathrm{PC}(u,v)$ starts at $v$ and traverses all the vertices of $G[J_2]$. The second path starts at $u$, traverses all the vertices of $G[J_1]$, $x$, and all the vertices of $GQ_2]$. 
\item 
Suppose that $v \in J_1$. 
\begin{itemize}
\item 
If $v$ is the only neighbour of $x$ in $G[J_1]$, $|J_1| > 1$, and $u'$ is the only neighbour of $u$ and $x$ in $G[J_2]$, then the condition (d) of this theorem would be violated. 
\item 
If $v$ is not the only neighbour of $x$ in $G[J_1]$ or $v$ is the only neighbour of $x$ in $G[J_1]$ and $|J_1| = 1$, then one path $\mathrm{PC}(u,v)$ starts at $v$, and traverses all other vertices of $G[J_1]$, $x$, and all vertices in $G[Q_2]$ and the second path starts at $u$ and traverses all vertices of $G[J_2]$. 
\item 
If $u'$ is not the only neighbour of $u$ and $x$ in $G[J_2]$, then one path $\mathrm{PC}(u,v)$ starts at $v$, and traverses all other vertices of $G[J_1]$, and the second path starts at $u$, traverses all vertices of $G[J_2]$, $x$, and all vertices in $G[Q_2]$. 
\end{itemize}
\end{itemize}

\textit{Case 2e. The condition (f) of Theorem~\ref{thm:4k1_1con} is violated.} Suppose that the conditions (a)-(e) of Theorem~\ref{thm:4k1_1con} hold. There exists a minimal vertex cut $\{x,y\}$ of $G$ such that $c(G-\{x,y\})=2$ (thus $G$ is 2-connected). Denote by $Q_1$ a component of $G-\{x,y\}$ which is a clique and by $Q_2$ the other component of $G-\{x,y\}$. Suppose that all neighbours of $x$ in $Q_2$ are articulation points of $G[Q_2]$ and $u = y$. 

The vertex $x$ must be adjacent to all the vertices in $Q_1$, otherwise we obtain $4K_1$. Suppose that $w$ is an articulation point of $G[Q_2]$ and denote the components of $G[Q_2]-\{w\}$ by $J_1$, $J_2$. 
The vertex $u$ has a neighbour in both $J_1, J_2$ since $G$ is 2-connected and at least one of them is not an articulation point of $G[Q_2]$. Several cases can occur depending on position of $v$. 
\begin{itemize}
\item 
If $v \in Q_1$, then we can obtain one path starting at vertex $v$, traversing all the vertices of $G[Q_1]$, and $x$. We obtain the second path by concatenating $u$ and a Hamiltonian path of $G[Q_2]$ starting in a neighbour of $u$ which is not an articulation point. 
\item 
If $v \in Q_2$ and $v$ is not an articulation point of $G[Q_2]$, then we can obtain one path starting at vertex $u$, traversing all the vertices of $G[Q_1]$, and $x$. The second path is a Hamiltonian path of $G[Q_2]$ starting in $v$.
\item 
If $v \in Q_2$, $v$ is an articulation point of $G[Q_2]$ and it is the only neighbour of $x$ in $G[Q_2]$, then $\{u,v\}$ would violate the condition (c) of this theorem. 
\item
If $v \in Q_2$, $v$ is an articulation point of $G[Q_2]$ and $x' \neq v$ is a neighbour of $x$ in $G[Q_2]$. The vertex $x'$ is also an articulation point of $G[Q_2]$, $v$ is adjacent to all vertices in at least one component, without loss of generality in $J_1$, and $x'$ is adjacent to all vertices in $J_2$. We obtain one path staring at $u$, traversing all the vertices of $G[Q_1]$, $x$, $x'$, and all the vertices of $G[J_2]$. The second path starts at $v$ and traverses all the vertices of $G[J_1]$. 
\end{itemize}
This concludes the proof in the case that $G$ is connected. 

Suppose that $G$ is not connected. Using Theorem~\ref{thm:3K1u}, the proof of this case follows. 
\end{proof}

\subsection{$5K_1$-free graphs}

We will start with full proof of Theorem~\ref{thm:5k1}.

\begin{proof}\textbf{of Theorem~\ref{thm:5k1}.}
We will use notation $N_Q(x)=\{y:y\in Q \wedge xy\in E(G)\}$ for a vertex $x\in V(G)$ and a set $Q$ of vertices of $G$.

If any of the conditions is violated, then $G$ does not have a Hamiltonian path. Suppose that all of the conditions are satisfied. We will show that then $G$ has a Hamiltonian path. 
  
\textit{Case 1. Suppose that $G$ is connected, but not $2$-connected.}
If there exists an articulation point such that $c(G-\{x\}) \geq 3$, then there is no Hamiltonian path. Suppose that for every articulation point $x$, $c(G-\{x\}) \leq 2$. 
Let $x$ be a fixed articulation point of $G$ and $Q_1, Q_2$ are components of $G-\{x\}$. First suppose that one of the components of $G-\{x\}$ is clique (say $Q_1$) and the other component is $4K_1$-free graph (say $Q_2$). Clearly, $G$ has a Hamiltonian path if and only if there exists a neighbour $u\in Q_2$ of $x$  such that there exists a Hamiltonian path of $G[Q_2]$ starting in $u$.

If both $Q_1$, $Q_2$ induce $3K_1$-free graphs, then $G$ has a Hamiltonian path if and only if $x$ has a neighbour  $ x_1 \in Q_1$ and a neighbour $x_2 \in Q_2$ such that they are not articulation points. If $x$ is adjacent only to articulation points in $G[Q_1]$ or in $G[Q_2]$, then condition (a) or (b) would be violated.
\textit{Case 2. Suppose that $G$ is $2$-connected, but not $3$-connected.}
If there is a vertex cut $\{x,y\}$ of size 2 in $G$ such that $c(G-\{x,y\}) > 3$, then $G$ does not have a Hamiltonian path. 

If there is a vertex cut $\{x,y\}$ of size 2 in $G$ such that $c(G-\{x,y\}) = 3$, then two components of $G-\{x,y\}$ are cliques, say $Q_1,Q_2$,  and the third component, say $Q_3$, induces a $3K_1$-free graph. In this case, $G$ has a Hamiltonian path if and only if there is a vertex in ${Q_3}$ which is not an articulation point of $G[Q_3]$ and which is adjacent to $x$  or $y$. Such vertex always exists since $G$ is $2$-connected.

Suppose from now on that for every vertex cut $\{x,y\}$ of size 2 in $G$, $c(G-\{x,y\})= 2$. Take some fixed vertex cut $\{x,y\}$ in $G$ and let $Q_1,Q_2$ be the two components of $G-\{x,y\}$.

\textit{Case 2a. Both $Q_1,Q_2$ induce $3K_1$-free graphs.}  

First suppose that $xy$ is not an edge $G$. Since $3K_1$-free graphs have path covers of size two starting at any pair of vertices by Theorem \ref{thm:3K1pathcover}, $G$ has a Hamiltonian path if and only if   at least one of $G[Q_1]$ and $G[Q_2]$ have a Hamiltonian path  starting 
in a neighbour of $x$ and ending in a neighbour of $y$. If this is not the case, then several cases can depending on which of the conditions (a)--(c) of Theorem \ref{thm:3K1_uv} is violated. 
\begin{itemize}
\item Condition (a) of Theorem \ref{thm:3K1_uv} is violated.
\begin{itemize}
\item 
If $N_{Q_1}(x) \cup N_{Q_1}(y)$ contains only articulation points of $G[Q_1]$, or $N_{Q_2}(x) \cup N_{Q_2}(y)$ contains only articulation points of $G[Q_2]$, then these are also articulation points in $G$ which is not possible.
\item 
If $N_{Q_1}(x)$ and $ N_{Q_2}(x)$ contain only articulation points of $G[Q_1]$ or $G[Q_2]$, respectively, then $x$ together with one vertex from each component of $G - (\{x,y\} \cup N_{Q_1}(x) \cup N_{Q_2}(x))$ would create $5K_1$. 
\item 
If $N_{Q_1}(x)$ and $ N_{Q_2}(y)$ (or analogously $N_{Q_1}(y)$ and $ N_{Q_2}(x)$) contain only articulation points, then we can obtain a Hamiltonian path firstly going through 
\begin{itemize}
\item all vertices of one clique in $Q_1$, 
\item the vertex $y$, 
\item all vertices in the second clique of $Q_1$,  
\item articulation point of $Q_1$ adjacent to $x$, 
\item the vertex $x$, 
\item a vertex in $N_{Q_2}(x)$ which is not an articulation point of $Q_2$, and
\item  a Hamiltonian path of $Q_2$ starting at vertex. 
\end{itemize} 
\end{itemize}
\item  Condition (b) of Theorem \ref{thm:3K1_uv} is violated.
If there is an articulation point $z$ in $Q_1$ (for $Q_2$ analogously) such that $N_{Q_1}(x) \cup N_{Q_1}(y)$ is a subset of one component of $G[Q_1] - \{z\}$ (possibly $z \in N_{Q_1}(x) \cup N_{Q_1}(y)$), then $z$ would be an articulation point also in $G$, which is not possible since $G$ is 2-connected.
\item Condition (c) of Theorem \ref{thm:3K1_uv} is violated.
If $N_{Q_1}(x) \cup N_{Q_1}(y)$ is a vertex cut of size 2 in $G[Q_1]$ (for $Q_2$ analogously), then it is also a vertex cut of size 2 in $G$ and after removing it, we get at least 3 components. 
\end{itemize}

If $xy$ is an edge, then a Hamiltonian path can be also obtained by concatenating a Hamiltonian path of $G[Q_1]$ starting in a vertex in $N_{Q_1}(x)$, $x$, $y$ and a Hamiltonian path of $G[Q_2]$ starting in a vertex in $N_{Q_2}(y)$ (or analogously with $x$ and $y$ interchanged).  A Hamiltonian path of $G[Q_1]$ starting in a vertex in $N_{Q_1}(x)$ and a Hamiltonian path of $G[Q_2]$ starting in a vertex in $N_{Q_2}(y)$ exist if and only if $N_{Q_1}(x)$ and $ N_{Q_2}(y)$ each contains a vertex which is not an articulation point. By a similar analysis we can prove that $N_{Q_1}(x)$ and $ N_{Q_2}(y)$ always contain such a vertex.

\textit{Case 2b. One of the components is a clique, say $Q_1$, and the other one, say $Q_2$, induces a $4K_1$-free graph.} 

Observe that $G$ has a Hamiltonian path if and only if there exits a path cover of size 2 in $G[Q_2]$ with one path starting at a vertex in $N_{Q_2}(x)$ and the second path starting in a vertex in $ N_{Q_2}(y)$. Such path cover does not exist if and only if
at least one condition of Theorem \ref{thm:4k1pc} is violated. Several cases can occur. 
\begin{itemize}
\item Condition (a) of Theorem \ref{thm:4k1pc} is violated.
First suppose that there is an articulation point $z$, such that $G[Q_2] -\{z\}$ has at least 3 components. If $N_{Q_2}(x)$ (or $N_{Q_2}(y)$)  contains only $z$, then $c(G-\{y,z\}) \geq 3$ (or $c(G-\{x,z\}) \geq 3$) which is not possible. Also,  $N_{Q_2}(x) \cup N_{Q_2}(y)$ cannot be a subset of one component of $G[Q_2] -\{z\}$ since $G$ is 2-connected. Thus,  $N_{Q_2}(x) \cup N_{Q_2}(y)$ contains vertices from different components of $G[Q_2] -\{z\}$ which are not articulation points of $G[Q_2]$.

\item Condition (b) of Theorem \ref{thm:4k1pc} is violated.
Suppose that there exists a triangle $x,y,z$ in $G$ such that $c(G-\{x,y,z\}) \geq 3$. Since $G$ is 2-connected, then $x$ or $y$ has a neighbour in $Q_2$ which is not an articulation point and $N_{Q_2}(x) \cup N_{Q_2}(y)$ cannot be a subset of one component of $G-\{x,y,z\}$.

\item Condition (c) of Theorem \ref{thm:4k1pc} is violated.
If $N_{Q_2}(x) \cup N_{Q_2}(y)$ is a vertex cut of size 2 in $G[Q_2]$, such that $c(G[Q_2] - (N_{Q_2}(x) \cup N_{Q_2}(y))) \geq 3$, then it is also a vertex cut in $G$ and  $c(G - (N_{Q_2}(x) \cup N_{Q_2}(y))) \geq 3$ which is not possible.

\item Condition (d) of Theorem \ref{thm:4k1pc} is violated.
In this case, there is an articulation point $w$ of $G$ such that $N_{Q_2}(x) \cup N_{Q_2}(y)$ is subset of only one component of $G-w$ which is not possible, since $G$ is 2-connected.

Therefore, in all cases, $G[Q_2]$ has a path cover with one path starting in a vertex in $N_{Q_2}(x)$ and the other one starting in a vertex in $ N_{Q_2}(y)$.
\end{itemize}

\textit{Case 3. $G$ is at least 3-connected.} Then it has a Hamiltonian path by Proposition~\ref{prop:chvatal}. 
\end{proof}

\begin{proof} \textbf{of Corollary~\ref{col:polytime}.}
A rough estimate of checking the conditions of Theorem~\ref{thm:4k1} comes out from first checking each  vertex $x\in V(G)$ whether it is an articulation point and what is the number of components of $G-\{x\}$ (this takes $O(n\cdot n^2)$ time) and then checking all triples of articulation points $x,y,z$ and the numbers of components of $G-\{x,y,z\}$ (this takes $O(n^2)$ time because a $4K_1$-free graph has at most 4 articulation points).

For $5K_1$-free graphs, the conditions are given by Theorems~\ref{thm:5k1} and subsequently by Theorem~\ref{thm:4k1_1con}. The most time costly is condition (c) of Theorem~\ref{thm:5k1}. After preprocessing the input graph and finding all articulation points in time $O(n^3)$, we check all of them (they are at most 6 of them, since $G$ is $5K_1$-free) and inspect the non-complete components for the existence of a suitable neighbour $u$ of the articulation point. We have $O(n)$ candidates for this $u$.  The suitability is given by conditions of Theorem~\ref{thm:4k1_1con}. In there, the most time costly condition is (f), which requires checking two-vertex cuts which contain $u$, hence $O(n)$ candidates, and for each of them identifying the articulation points of the non-complete component and checking if the other vertex from he cut has a neighbor which is not an articulation. This takes $O(n^3\cdot n)$ time.
\end{proof}

\input{L21.tex}

\section{Conclusion with full details}\label{sec:Conclusion-detailed}

\subsection{Maximum linkages, longest paths}

An optimization version of the Hamiltonian path problem is looking for the maximum possible length of a path in the input graph, or the maximum length of a path connecting two specified vertices. A straightforward generalization to Hamiltonian linkages is the {\sc Maximum-$\ell$-Linkage} problem which asks for the maximum number of vertices that can be covered by a linkage of given $\ell$ pairs of vertices. Our Algorithm~\ref{alg:algorithm} can be modified to solve this optimization version in the following way.

Call the {\em defect} of a graph $G$ with respect to vertices $s_1,\ldots,s_{\ell},t_1,\ldots,t_{\ell}$, denoted by $\mbox{def}(G,\ell,s_1,\ldots,s_{\ell},t_1,\ldots,t_{\ell})$, the minimum number of vertices that remain uncovered by a linkage of the vertices $s_1,\ldots,s_{\ell},t_1,\ldots,t_{\ell}$ in $G$. Set  $\mbox{def}(G,\ell,s_1,\ldots,s_{\ell},t_1,\ldots,t_{\ell})-\infty$ if $G$ does not contain any linkage of  the vertices $s_1,\ldots,s_{\ell},t_1,\ldots,t_{\ell}$. Then the algorithm $\mbox{MinDefect}(G,k,\ell,s_1,\ldots,s_{\ell},t_1,\ldots,t_{\ell})$ which will return a value from $\mathbb{Z}^+\cup\{0,\infty\}$
%tu by som dala $\mathbb{Z}\cup\{0, \infty\}$ a prerobila som Mindefect na \mbox{MinDefect}, inak to chape ako m*i*n...
will run similarly as Algorithm~\ref{alg:algorithm}, with the following adjustments:

\begin{itemize}
\item The base case of $\ell=0$ is $\mbox{MinDefect}(G,k,0)\leftarrow |V(G)|$.
\item If $c_v(G)\ge g(k,\ell)$, we return $\mbox{MinDefect}(G,k,\ell,s_1,\ldots,t_{\ell})=0$.
\item A collection of scenarios is plausible if every vertex of the graph belongs to at most one of its scenarios.
\item We return $\mbox{MinDefect}(G,k,\ell,s_1,\ldots,t_{\ell})=\infty$ if there is no plausible collection of scenarios.
\item Instead of processing all scenario collections until finding one that allows a Hamiltonian linkage, we compare the defects $\mbox{Defect}(G,k,{\cal S})$ of all scenario collections and return the minimum one.
\item The defect with respect to one scenario collection $\cal S$ is computed recursively as
$$\mbox{Defect}(G,k,{\cal S})=|A\setminus\bigcup{\cal S}|+\sum_{i=1}^s \mbox{MinDefect}(G[Q'_i],k-1,\ell'_i,s'_i,\ldots,t'_i).$$  
\end{itemize} 
The running time is essentially the same as of Algorithm~\ref{alg:algorithm}, i.e., $O(n^{f(k,\ell)})$. By checking all possible $O(n^{2\ell})$ pairs of need-to-be-linked vertices, we can determine the maximum number of vertices that can be covered by $\ell$ disjoint paths in a $kK_1$-free graph $G$ in time $O(n^{2\ell+f(k,\ell)})$. By checking all pairs of adjacent vertices, we can determine the length of a longest cycle in time $O(n^{2+f(k,1)})$.   

\subsection{Constructing Hamiltonian linkages, paths and cycles}

If we are interested in the constructive versions of the problems, rather than only the decision ones, we can actually construct a maximum linkage in a similar running time. In the recursive calls we return the optimal linkages of the components $Q_i'$ instead of just the defect, and we concatenate them to an optimal linkage of entire $G$. 

Slightly more tricky is the case of highly connected input graphs. If $c_v(G)\ge g(k,\ell)$, we first construct a linkage of the input vertices via the method of~\cite{thomas2005improved}. Their proof of existence can be turned into a constructive one, the most costly part is finding a rigid separation, which can be done by brute force in $O(n^{2\ell})$ time. So altogether in $O^*(n^{2\ell})$ 
time we find a linkage of the need-to-be-linked vertices. Then we employ our proof of Theorem~\ref{thm:Ham-linked}. If the current linkage $P_1,\ldots,P_{\ell}$ does not contain all vertices, we pick a vertex $x$ uncovered by this linkage, find the paths $R_1,\ldots,R_m$ using network flow techniques in polynomial time and improve the linkage along the lines of the proof. This improving step needs to be repeated at most $n$ times.    
We conclude that the case of highly connected input graphs can be solved in $O^*(n^{2\ell})$ time. %tu tiez?
Since $f(k,\ell)\ge 2\ell$, the overall running time is upper bounded by the running time of the recursive case.

\subsection{Fixed parameter tractability}

From the Fixed Parameter Tractability point of view,  
our results can be restated so that {\sc Hamiltonian-$\ell$-Linkage}, {\sc Hamiltonian-$\ell$-Linkedness}, {\sc $\ell$-Path-Cover}, {\sc Maximum-$\ell$-Linkage} and {\sc Maximum-$\ell$-Path-Cover} are in the class XP when parameterized by $\ell$ and $\alpha(G)$. The natural question is the following.

\begin{problem}
Is any of these problems in FPT when parameterized by $\ell$ and/or $\alpha(G)$?
\end{problem}

The problems with bounded $\ell$, i.e., {\sc Hamiltonian-Path}, {\sc Hamiltonian-Cycle}, {\sc Hamiltonian-$1$-Linkage} and {\sc Path-Cover} are in the class XP when parameterized by $\alpha(G)$. Thus we ask the following question.

\begin{problem}
Is any of these problems in FPT when parameterized by $\alpha(G)$?
\end{problem}

This is also a good place to comment on an estimate of the function $f(k,\ell)$. A careful analysis of the recursion $f(k,\ell)\le 2g(k\ell)+f(k-1,g(k,\ell)+\ell)$ shows that $f(k,\ell)=O((k+1)!\cdot \ell)$. We omit the proof, since our primary goal was just to show that $f(k,\ell)< \infty$.

\subsection{Graphs with bounded tree independence number} 

A very recent approach in algorithmic applications of width parameters of graphs is the so called \emph{tree independence number}. 
Dallard, Milanič and Štorgel~\cite{dallard2021tree} define it in the following way. If 
 $\mathcal{T} = (T, \{ X_t \}_{t\in V(T)})$ is a tree decomposition of a graph $G$, the \emph{tree independence number} of $\cal{T}$  is defined as 
$$ \alpha(\mathcal{T}) = \mathrm{max}_{t \in V(T)} (\alpha(G[X_t])$$
and the tree independence number of $G$, denote by $\mathrm{tree-}\alpha(G)$ is the minimum tree independence number $ \alpha(\mathcal{T})$ among all possible tree decompositions $\mathcal{T}$ of $G$. They prove that several optimization problems are polynomial time solvable on graphs of bounded tree independence number.

However, the hope that our results could be extended to graphs of bounded tree independence number has vanished very quickly. 
Hamiltonian circuit and Hamiltonian path are NP-complete for chordal graphs, cf.~\cite{bertossi1986hamiltonian}, i.e., for graphs of tree independence number equal to 1.
